# Supplementary material for: SDF-SRN: Learning Signed Distance 3D Object Reconstruction from Static Images
Source: arXiv:2010.10505 source file (2020-10-20)
Supplement: Supplementary file 1 [file supp-pascal3d3c.pdf]

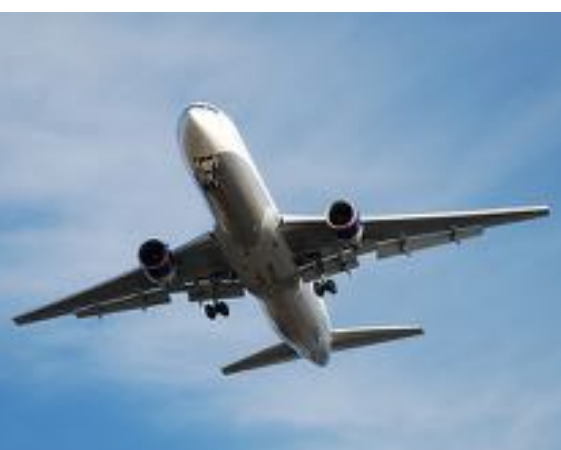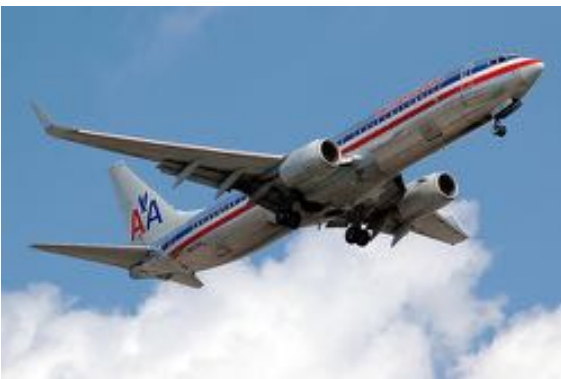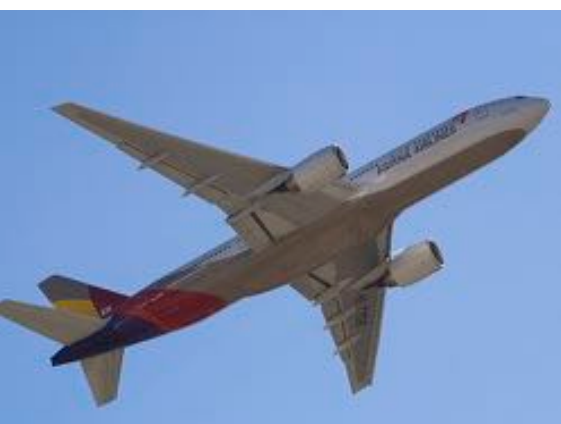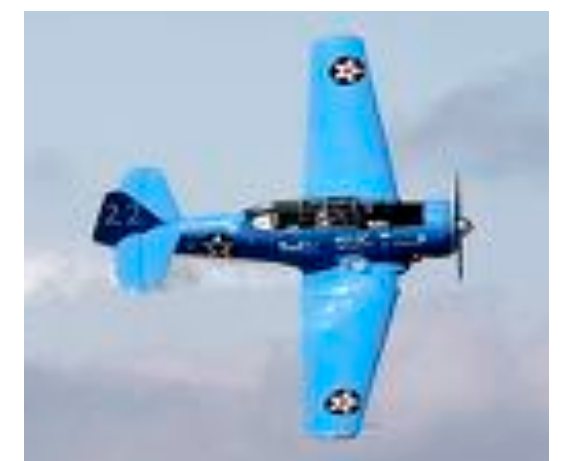

Input

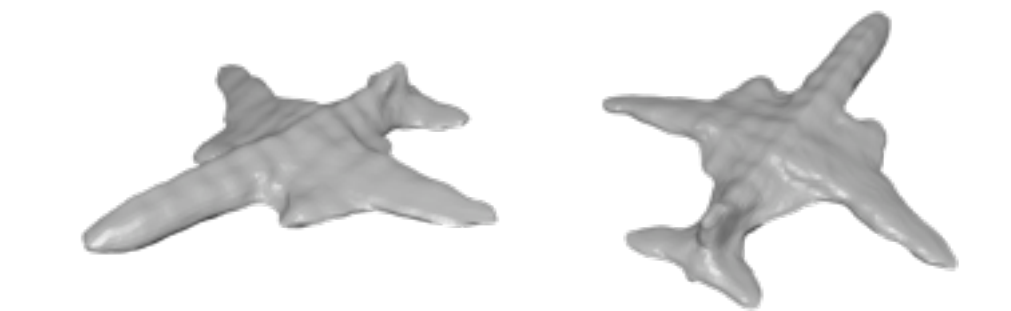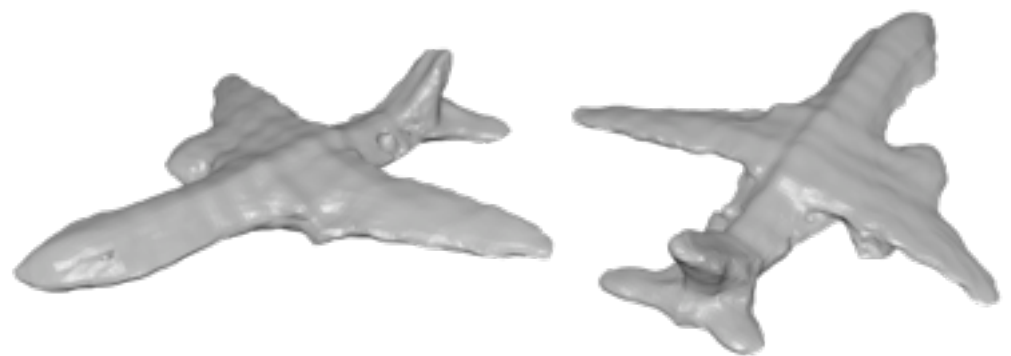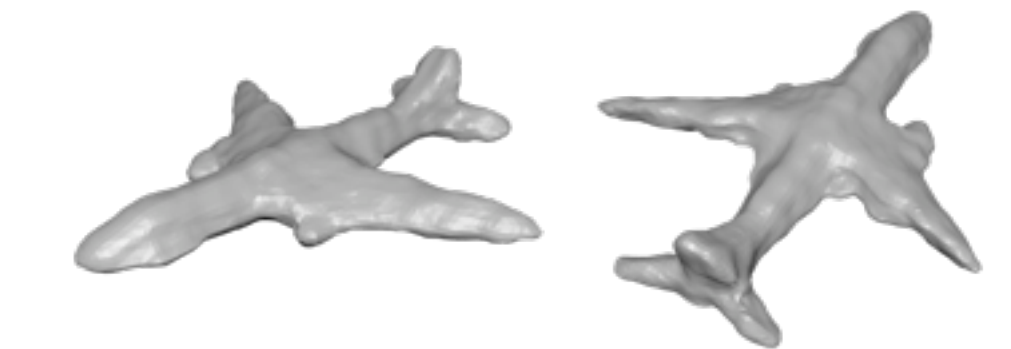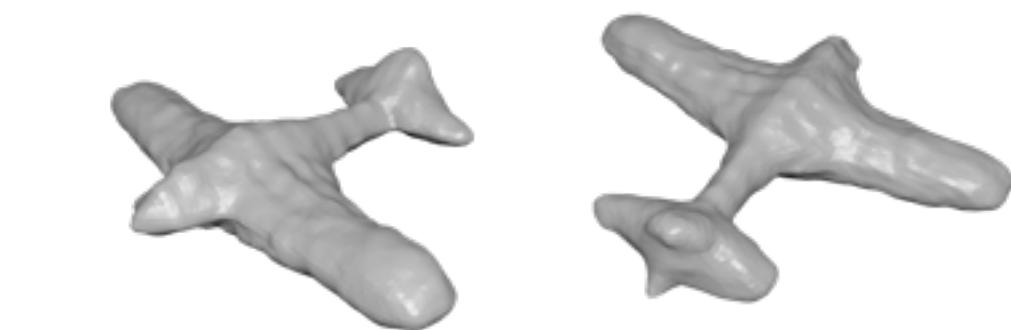

SDF-SRN (ours)

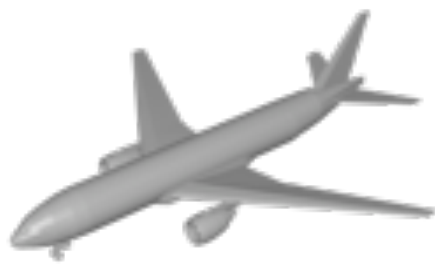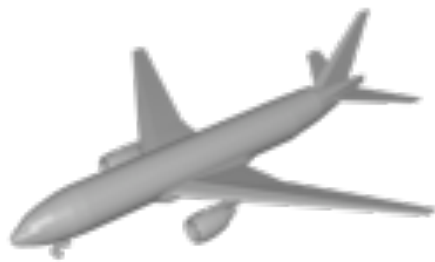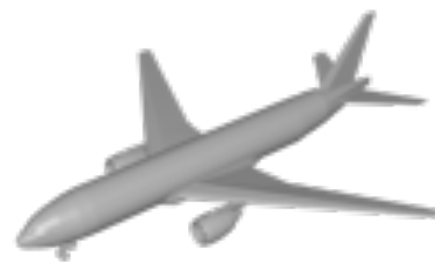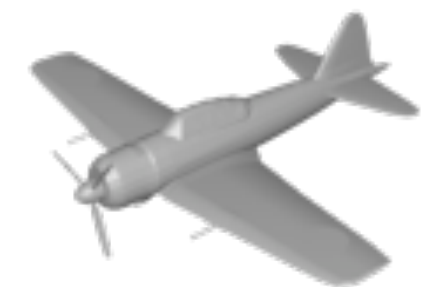

GT

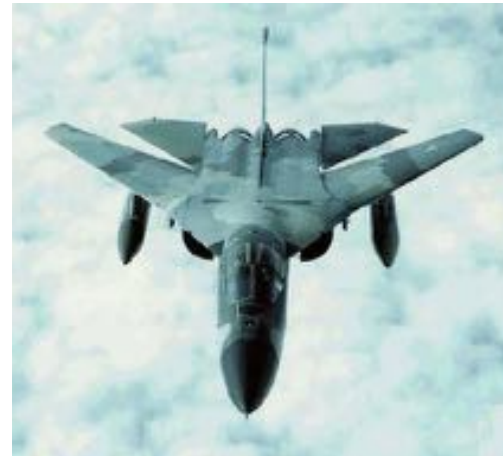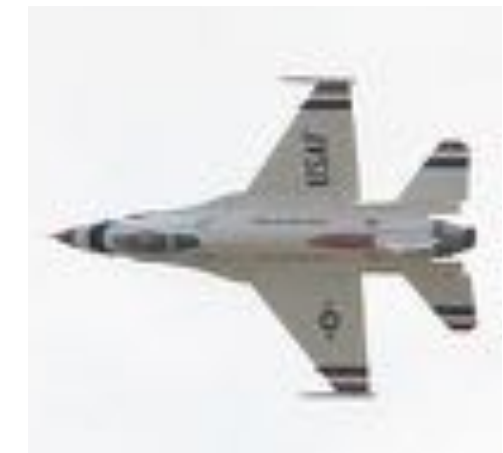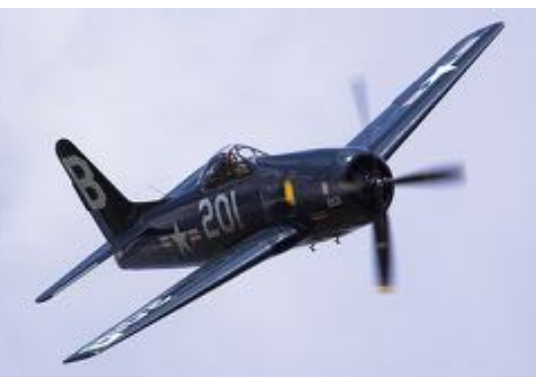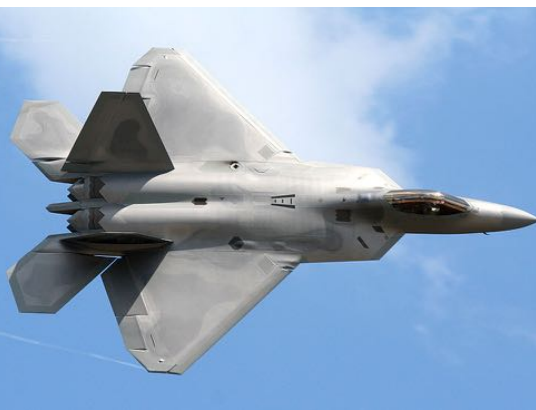

Input

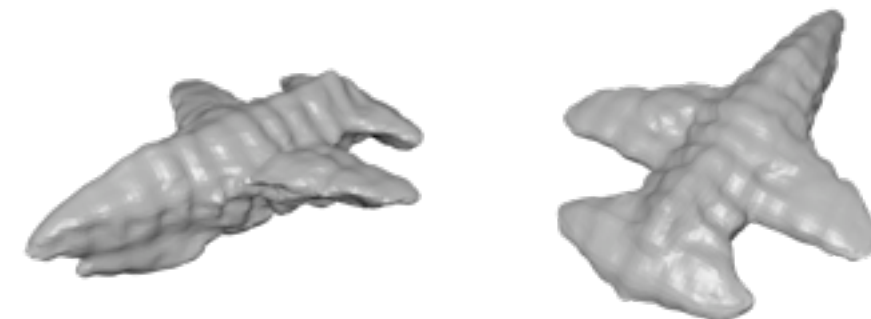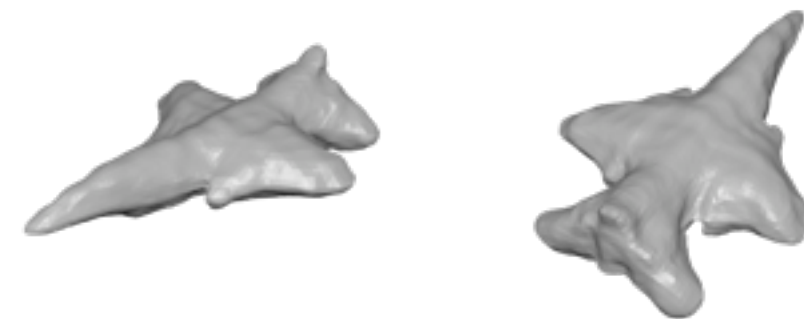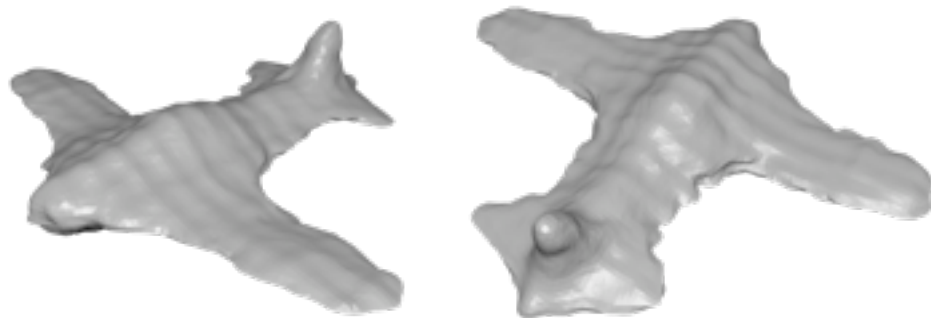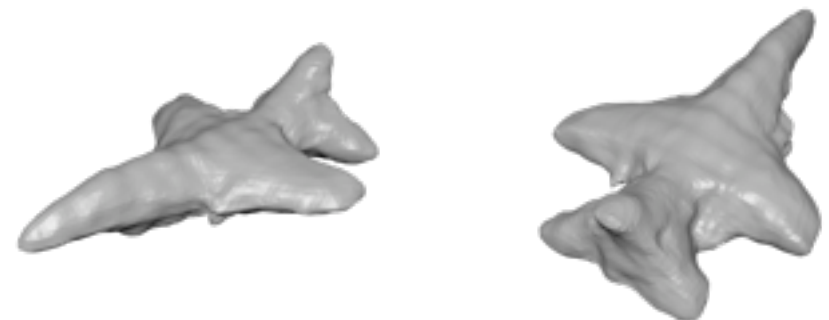

SDF-SRN (ours)

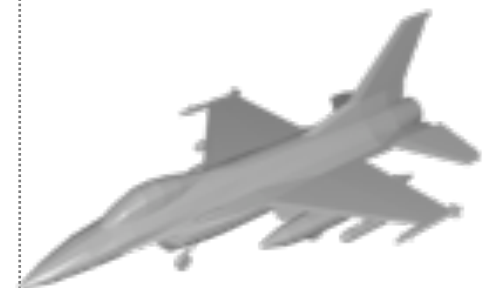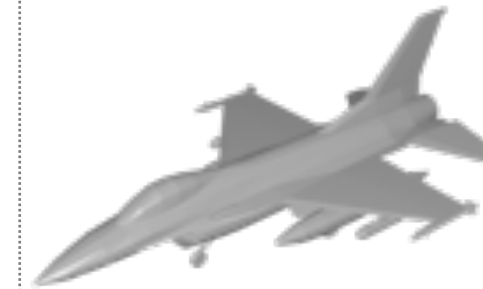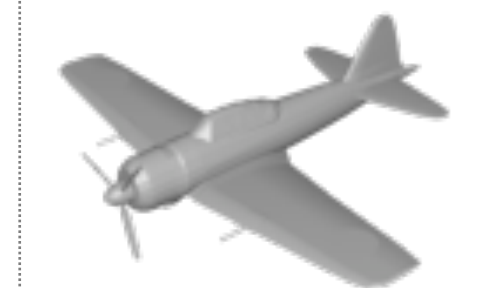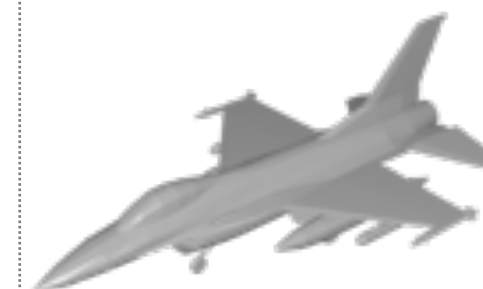

GT



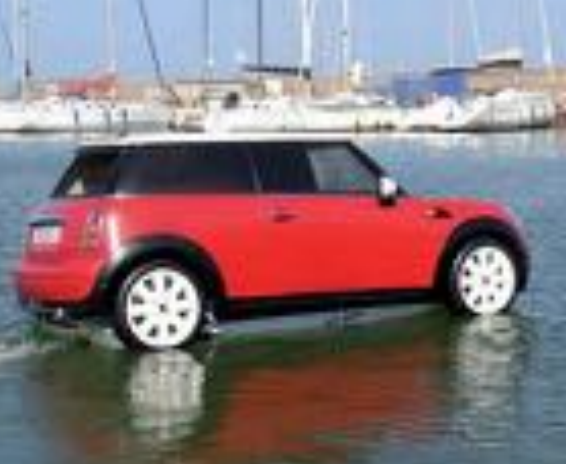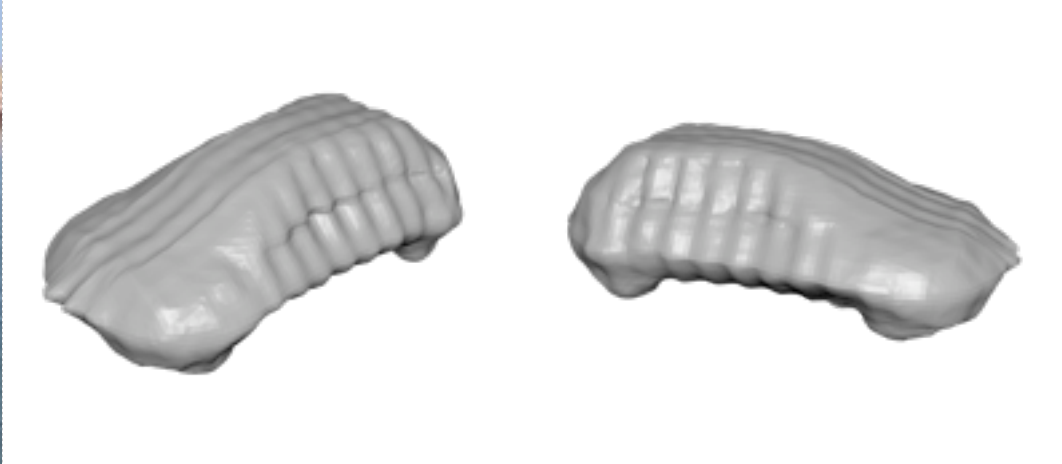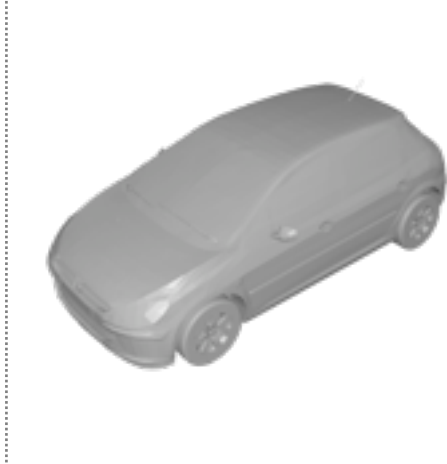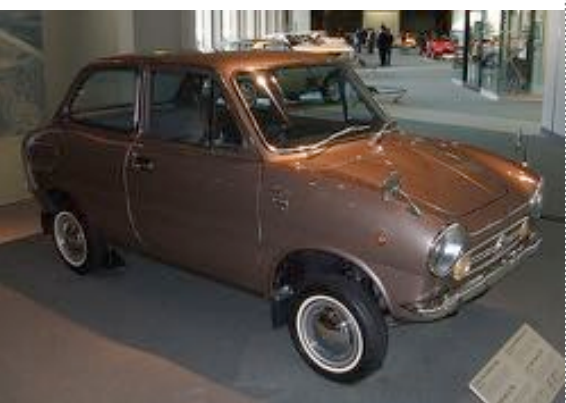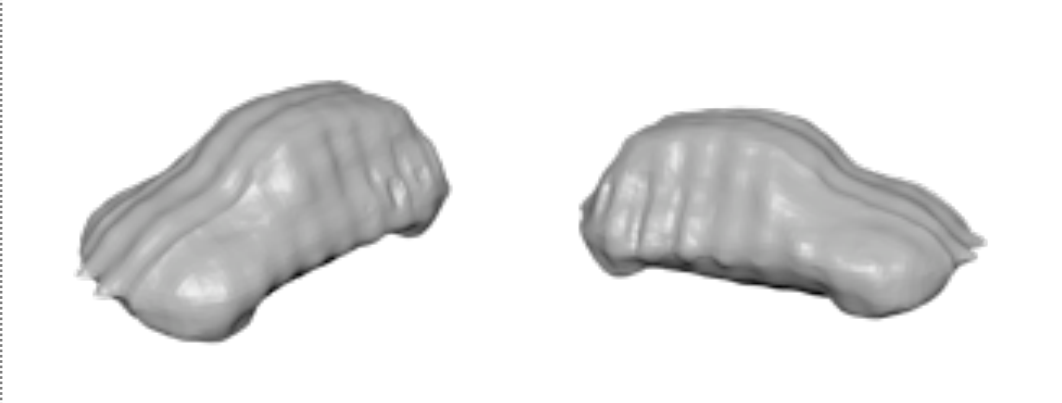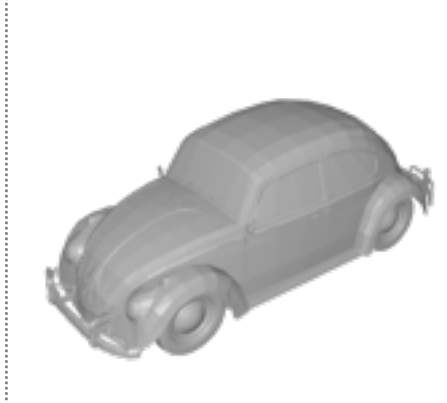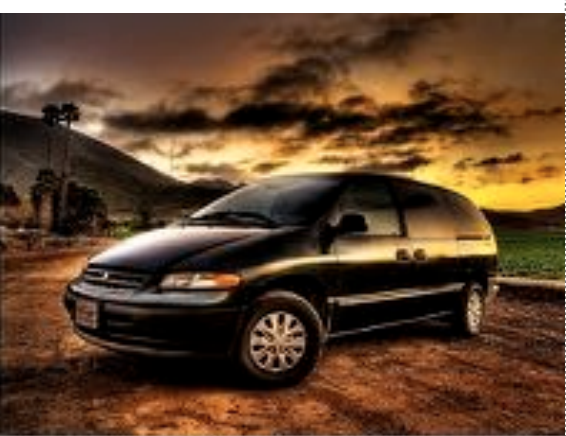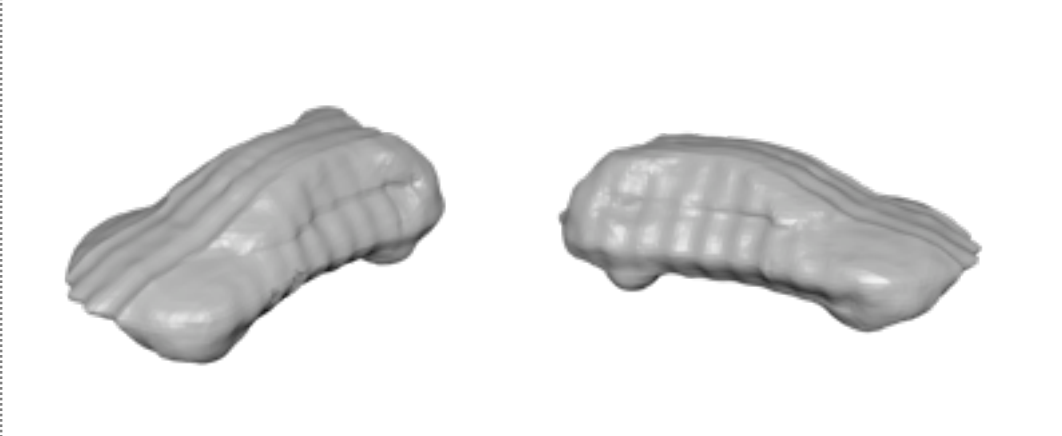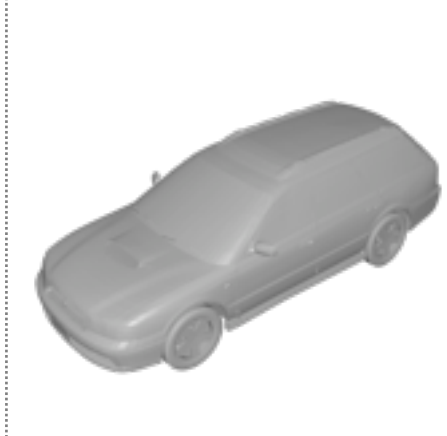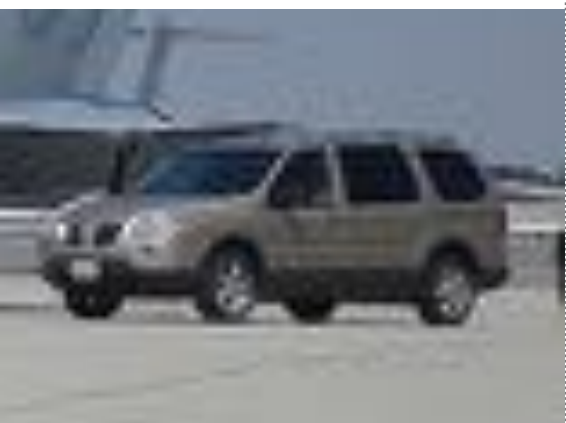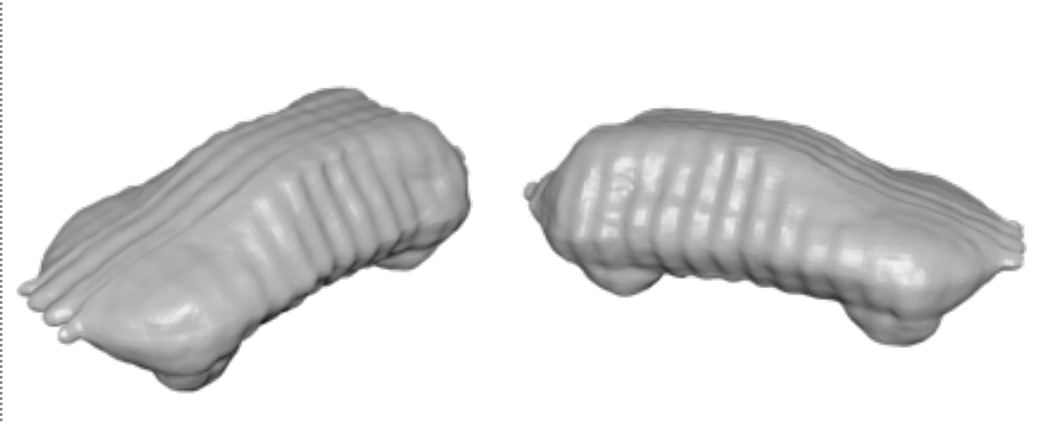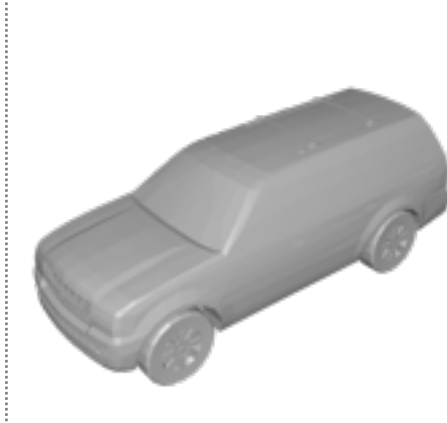

Input

SDF-SRN (ours)

GT

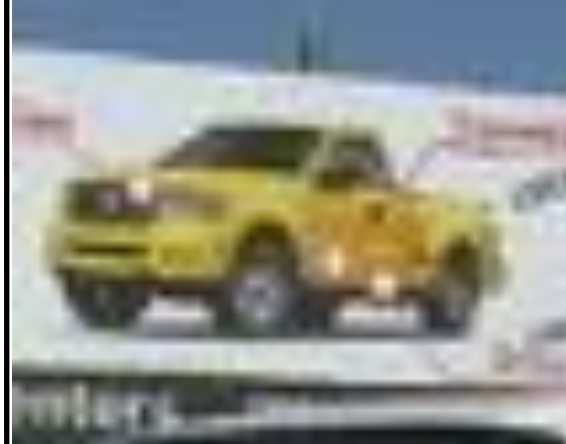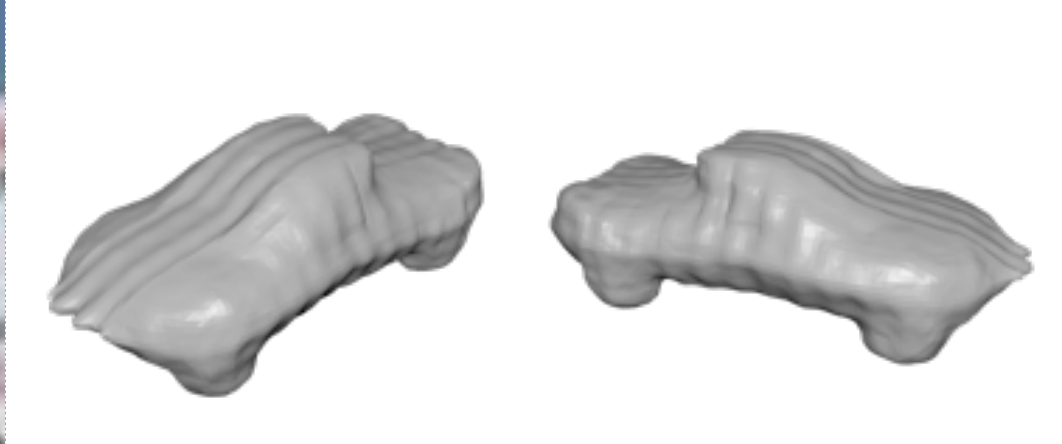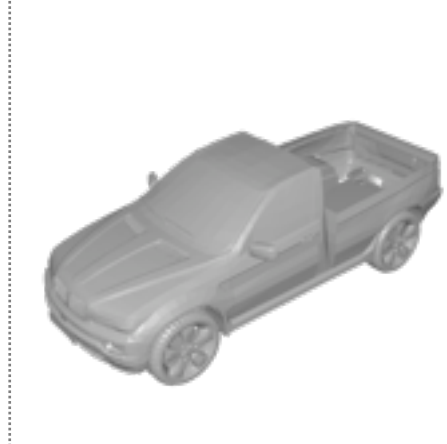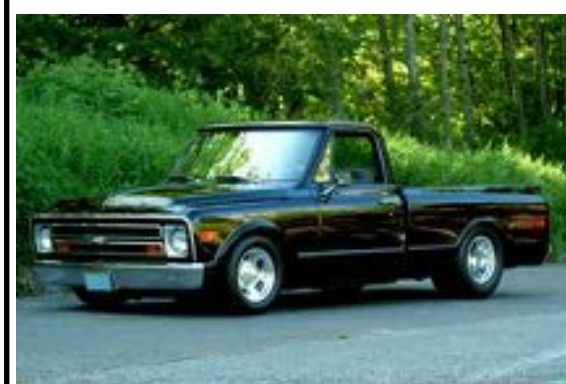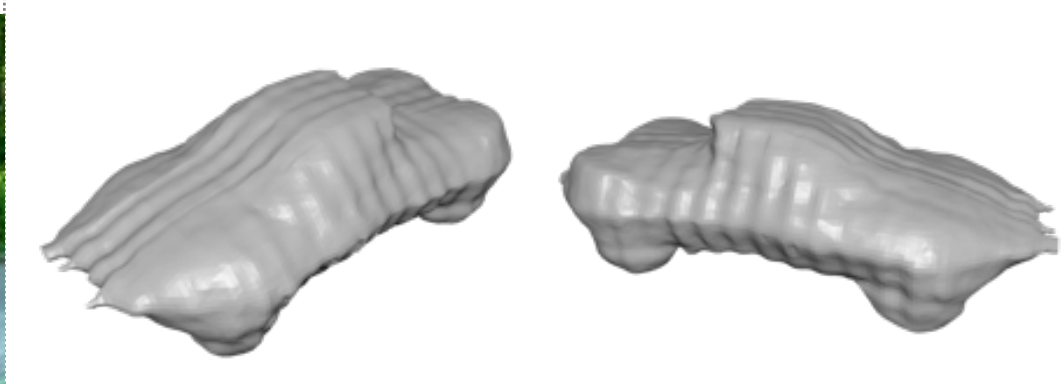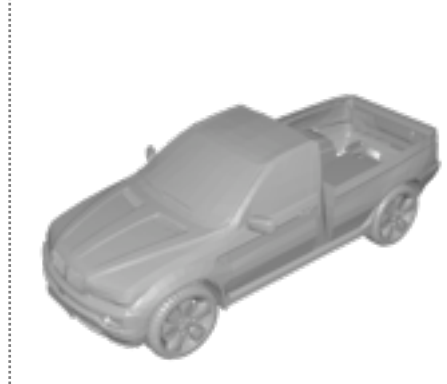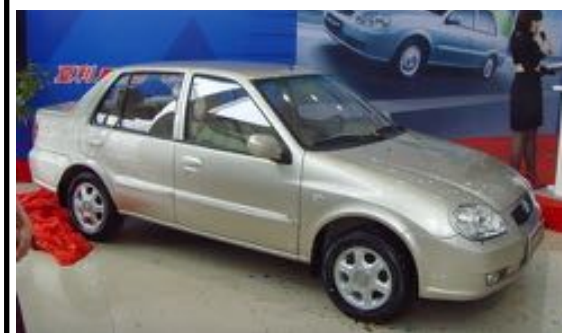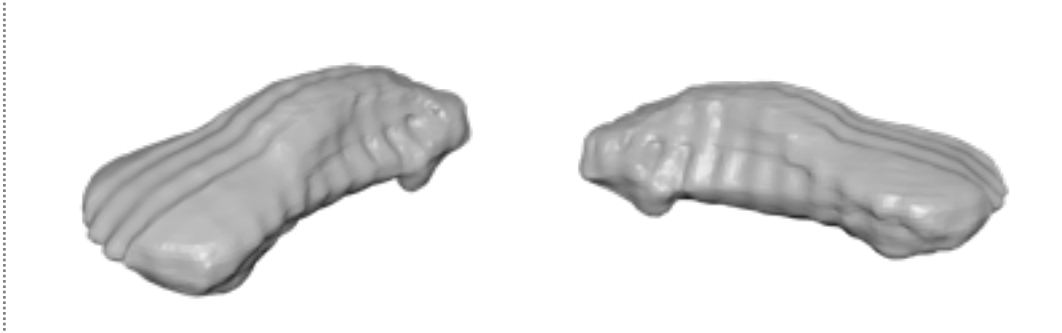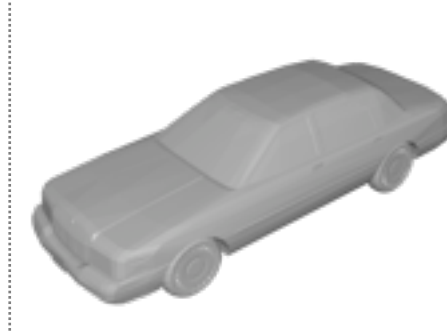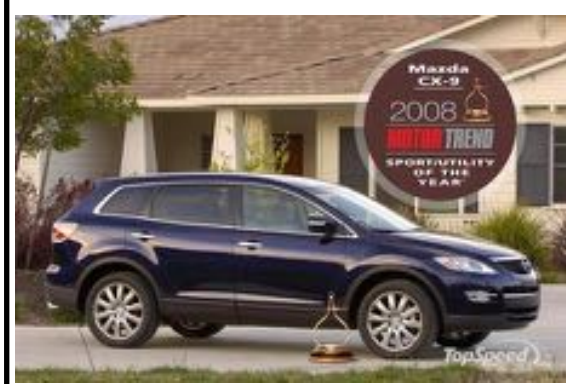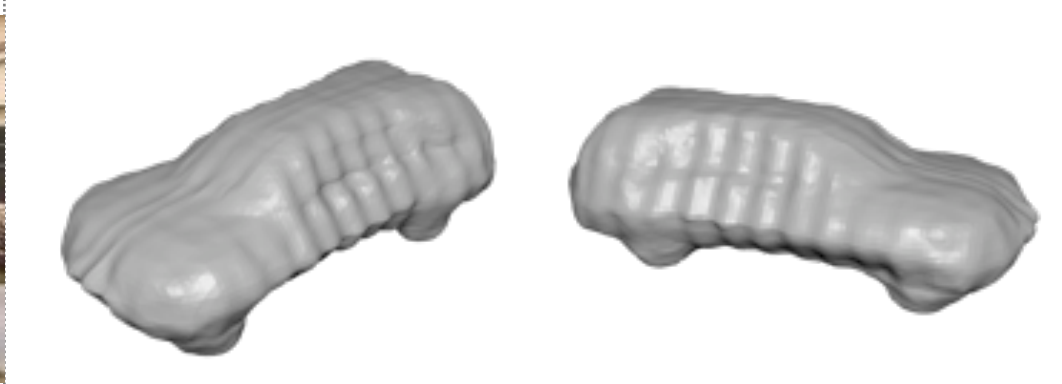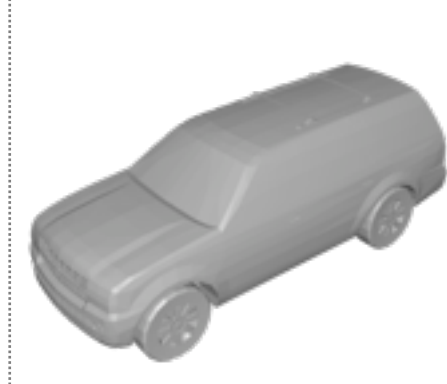

Input

SDF-SRN (ours)

GT



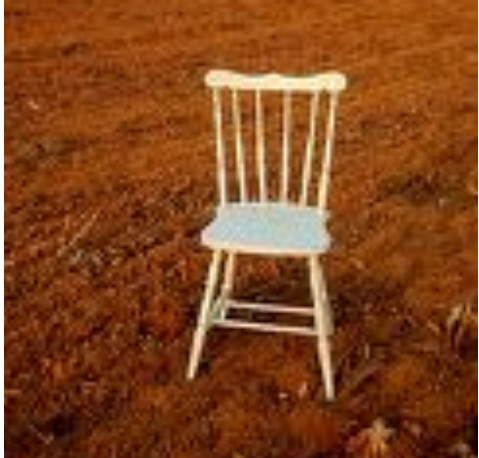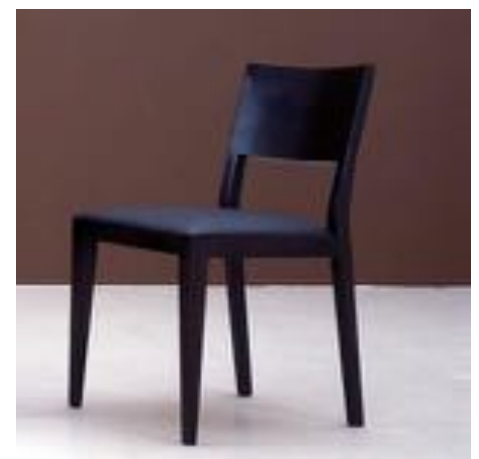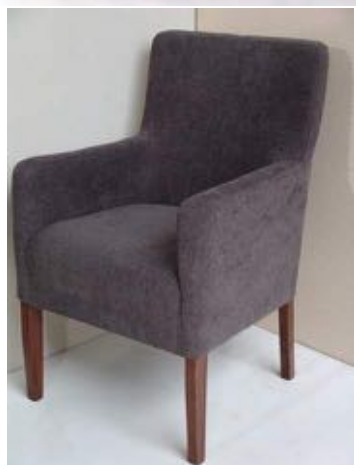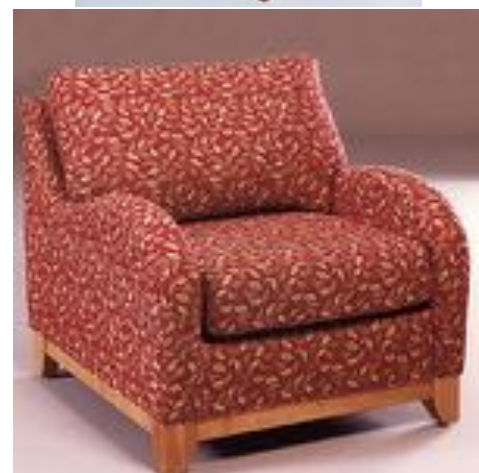

Input

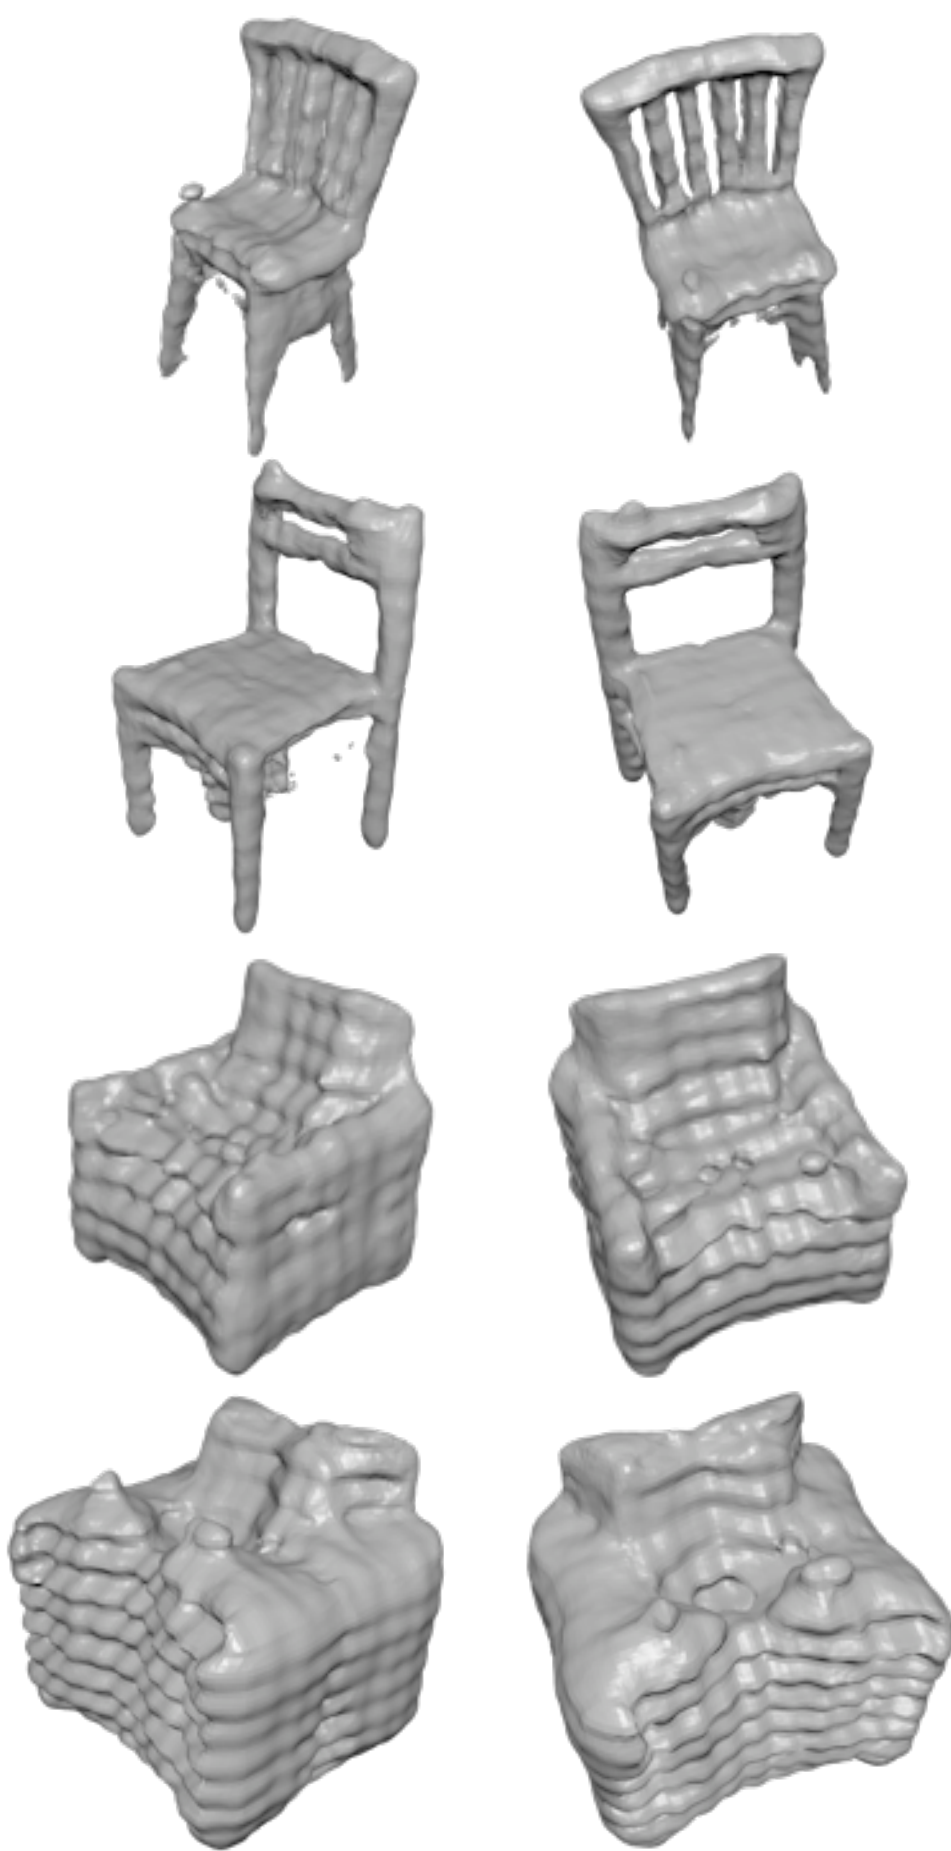

SDF-SRN (ours)

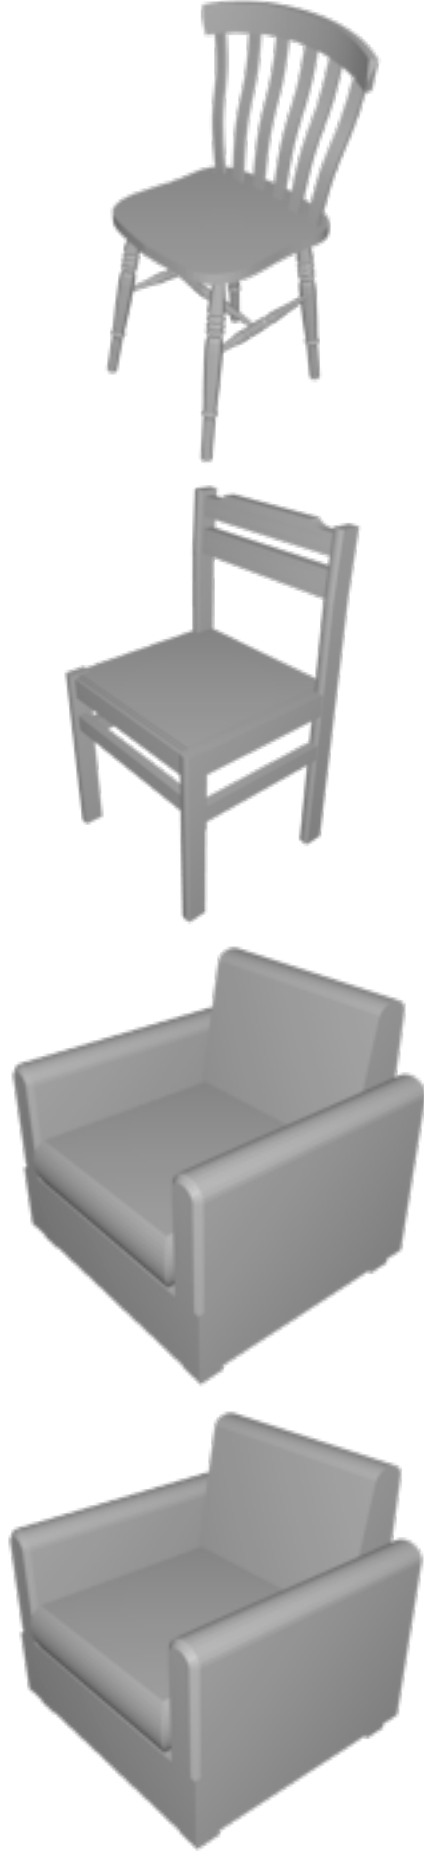

GT

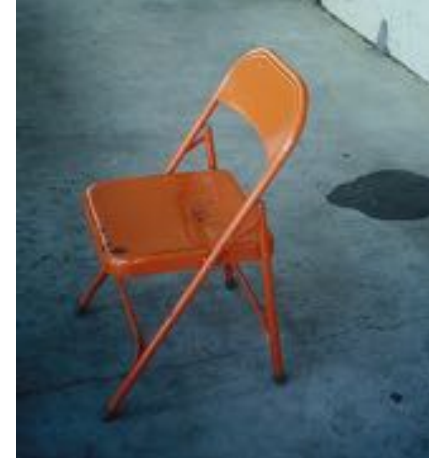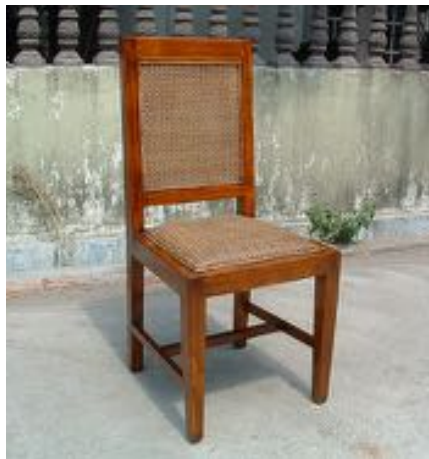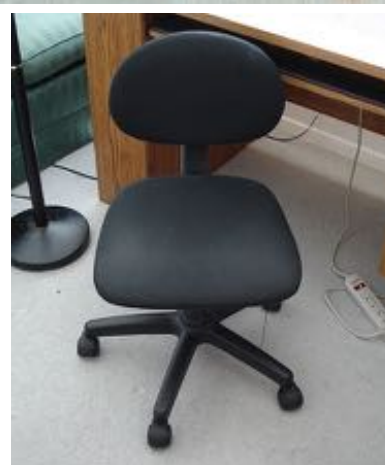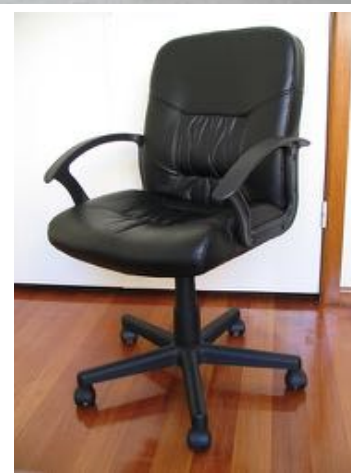

Input

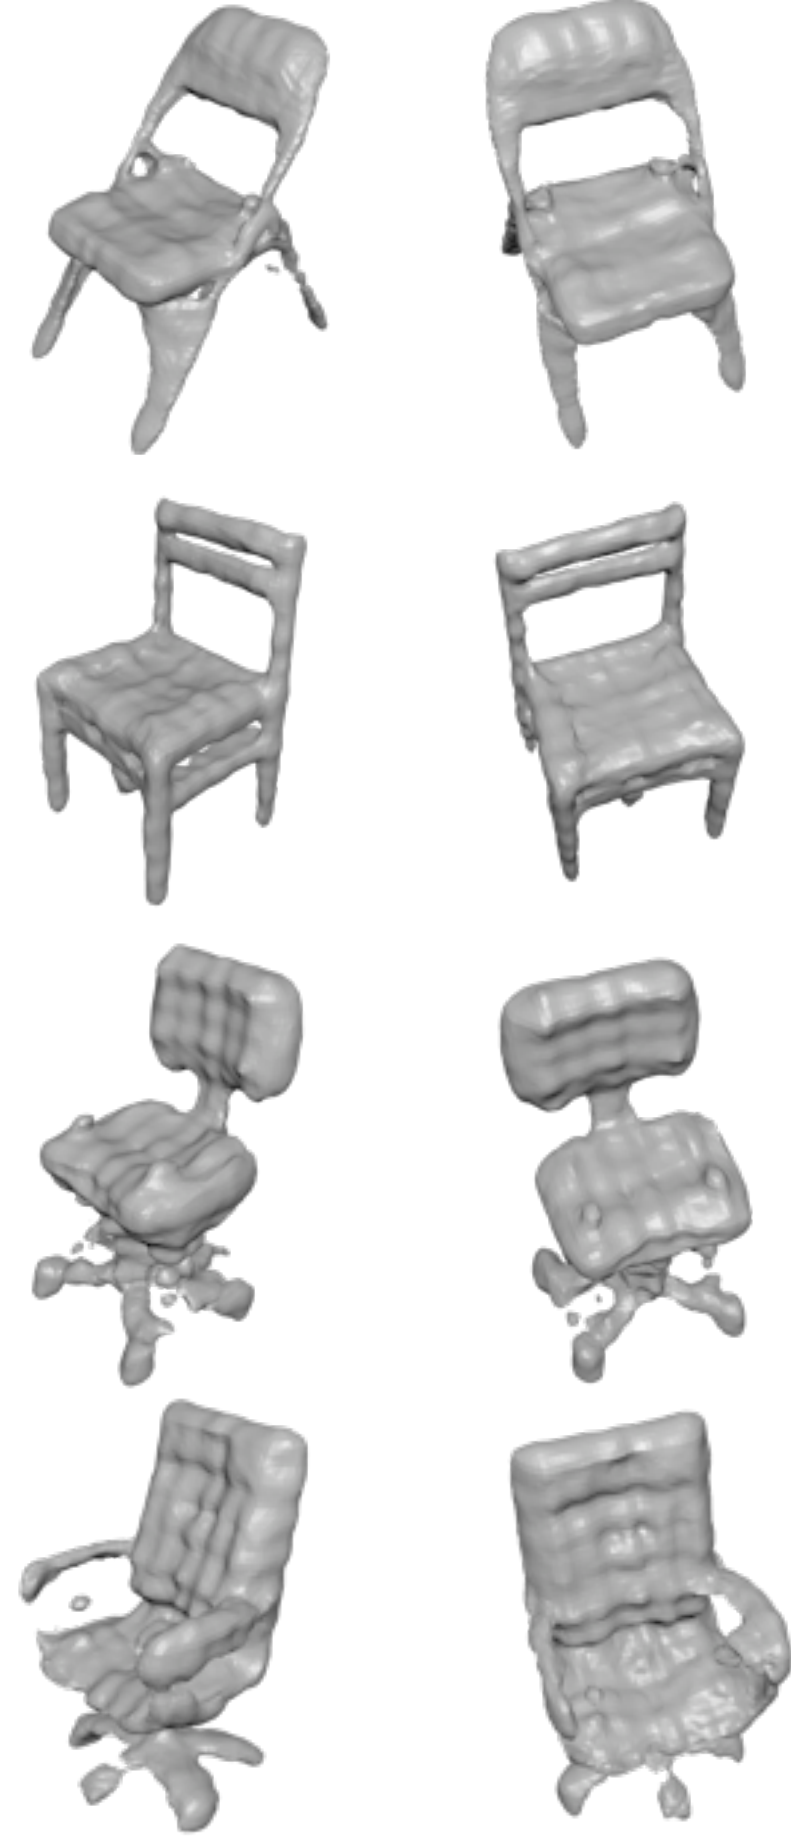

SDF-SRN (ours)

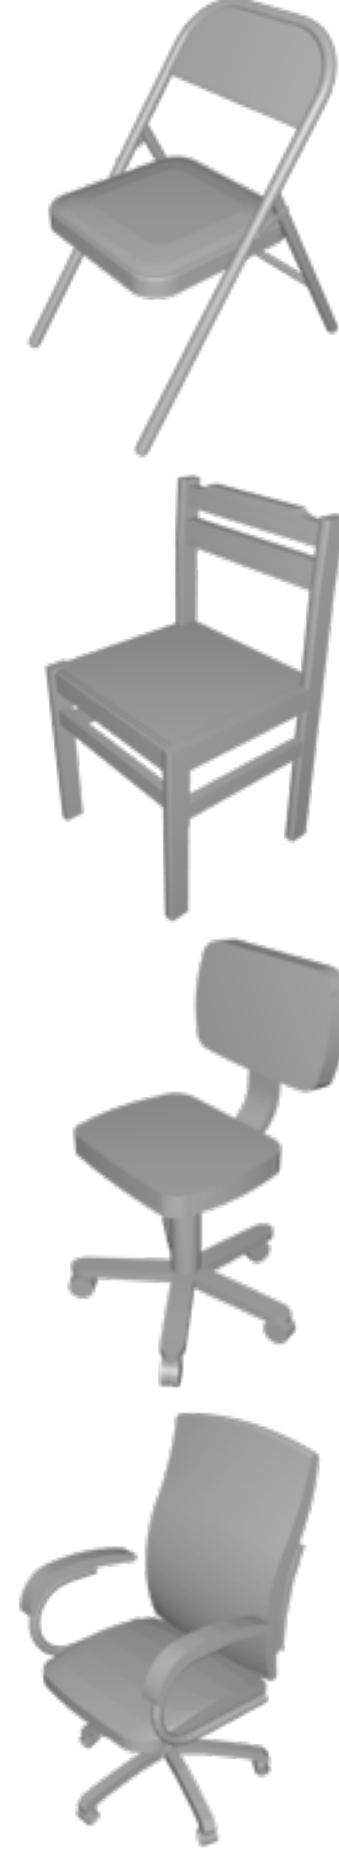

GT
