# Supplementary material for: SDF-SRN: Learning Signed Distance 3D Object Reconstruction from Static Images
Source: arXiv:2010.10505 source file (2020-10-20)

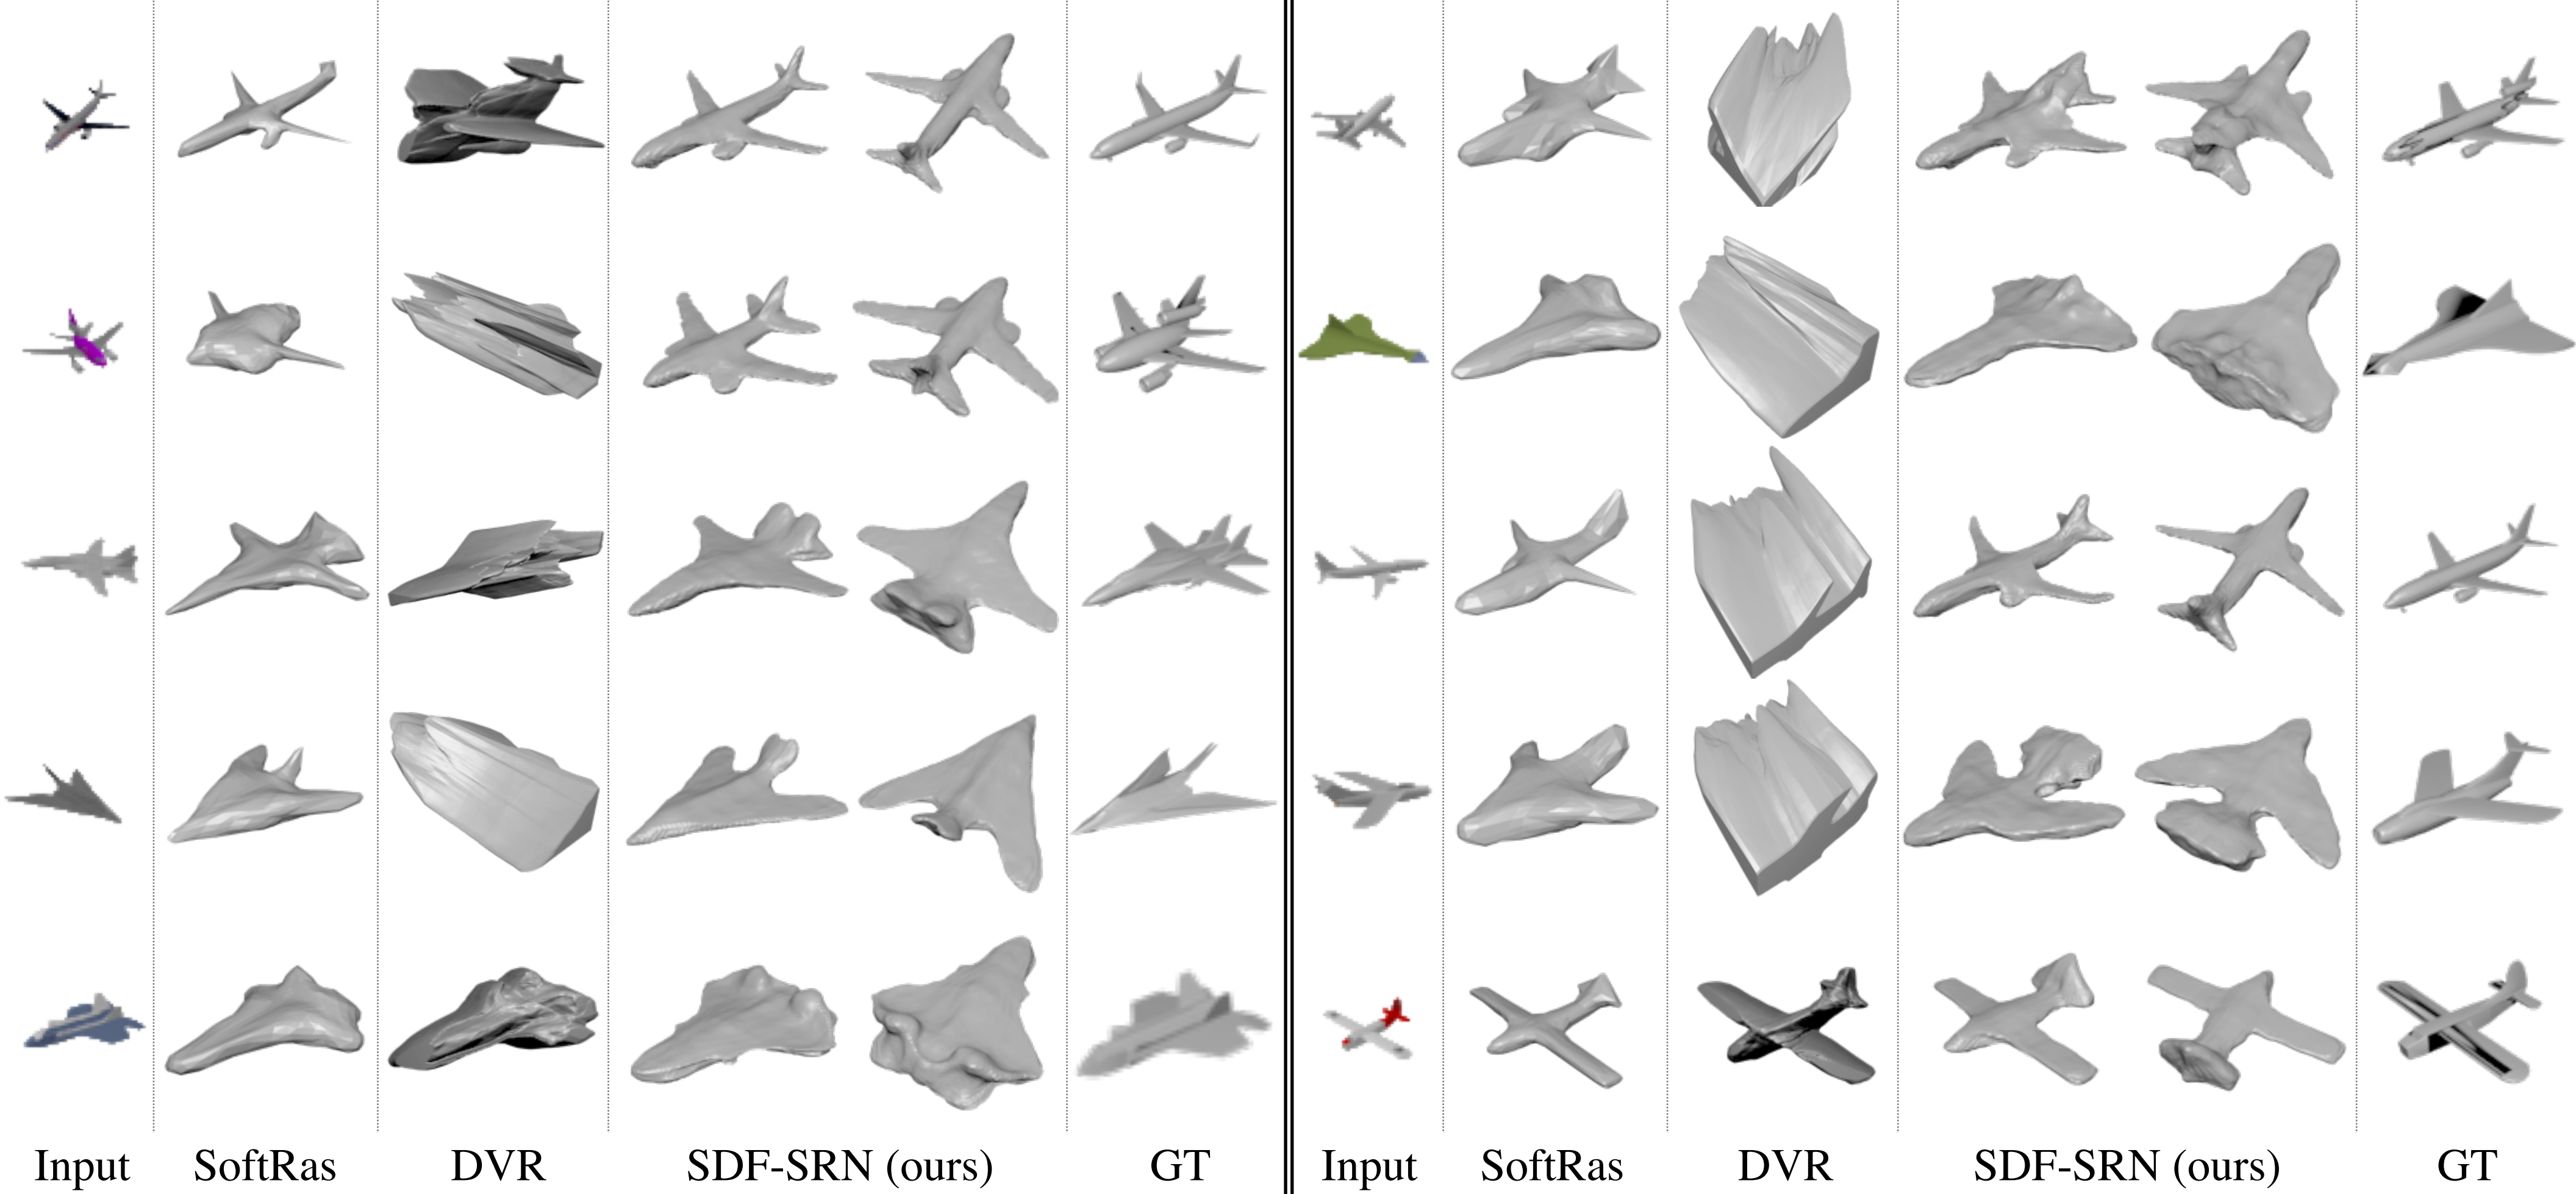

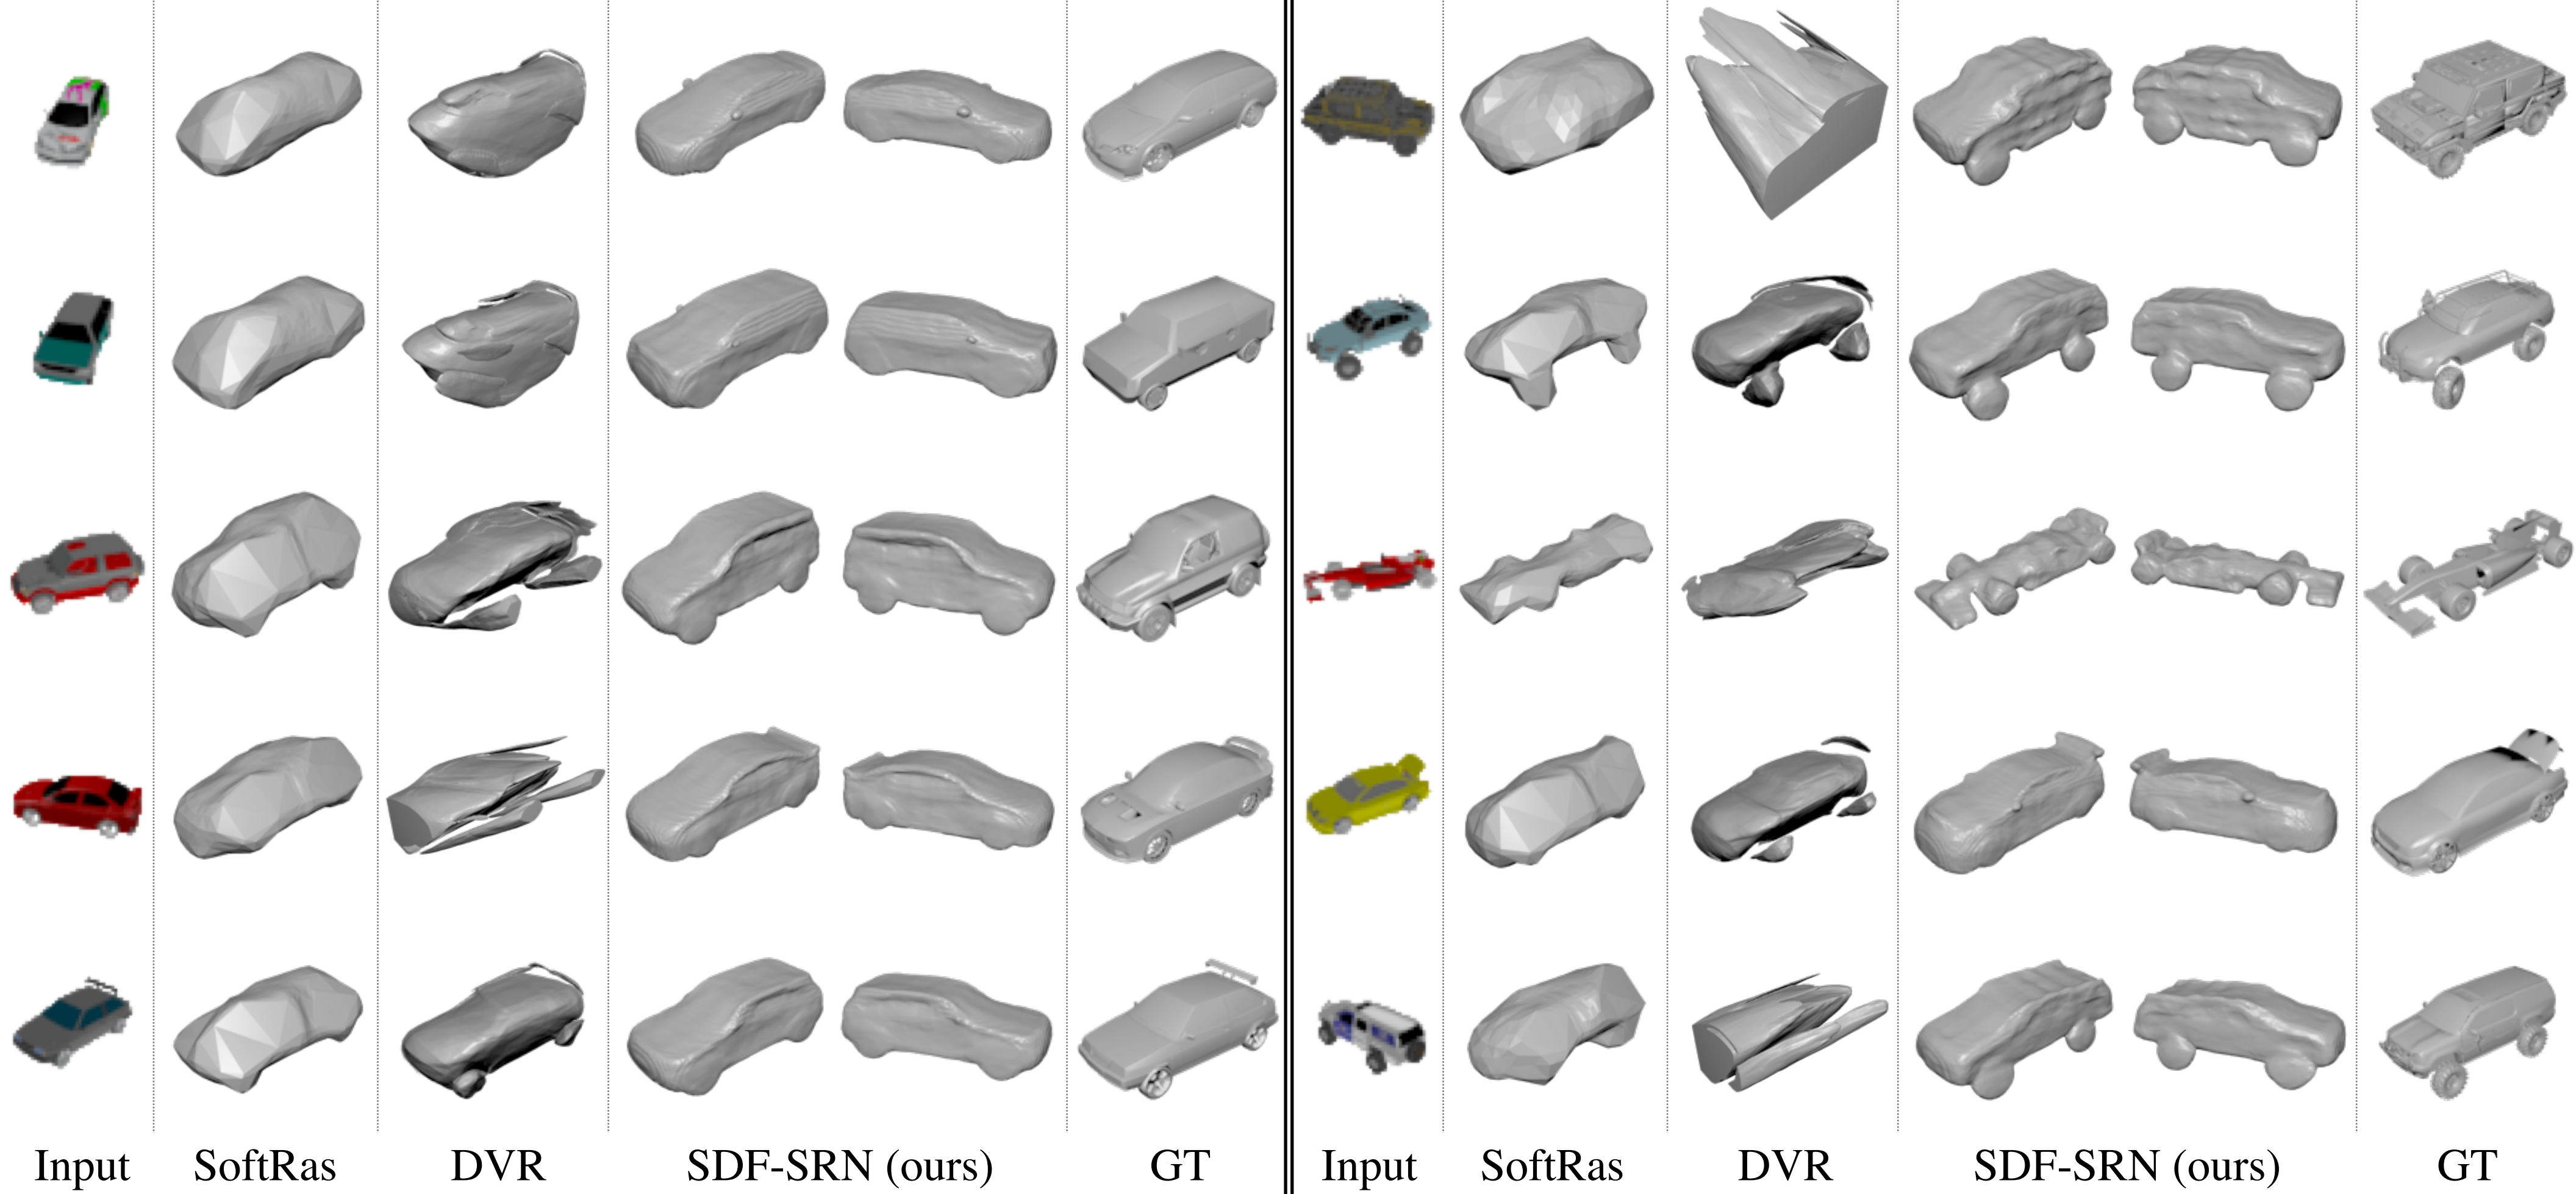



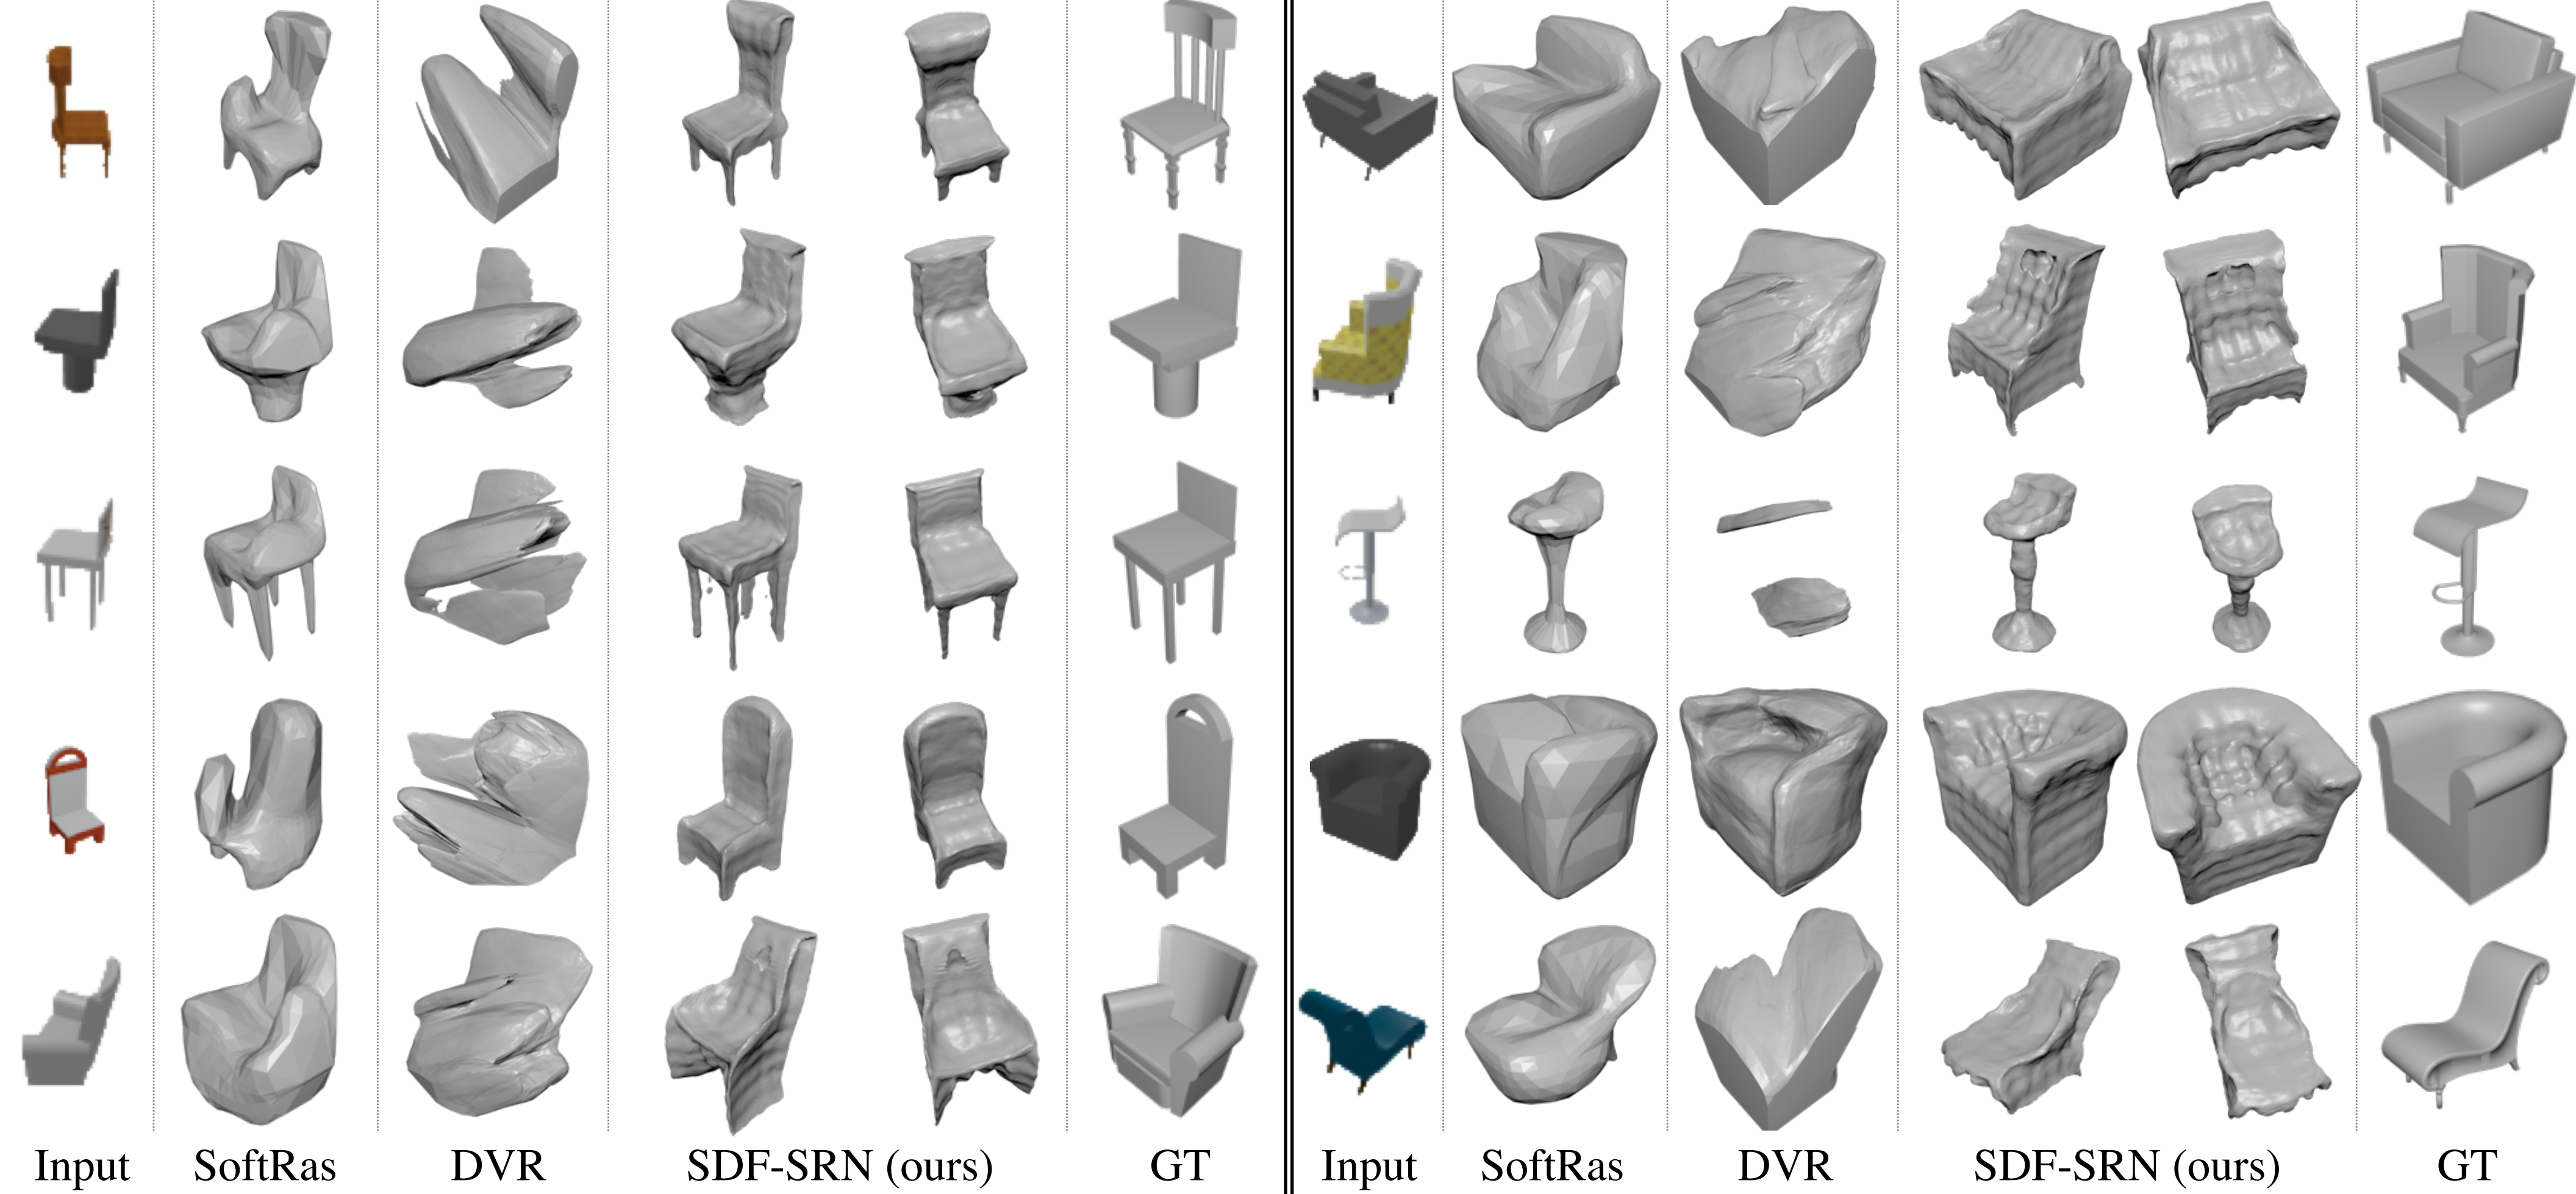

Supplement: Supplementary file 2 [file supp-shapenet2c.pdf]
